# Supplementary material for: Ultrafast dynamics of excited electronic states in nitrobenzene measured by ultrafast transient polarization spectroscopy
Source: arXiv:1912.12902 ancillary file (2019-12-30)
Supplement: Supplementary file 1 [file UTPS_arXiv_supp_submitted_20191230.pdf]

# Ultrafast dynamics of excited electronic states in nitrobenzene measured by ultrafast transient polarization spectroscopy:

## Supporting Information

Richard Thurston,<sup>1</sup> Matthew M. Brister,<sup>1</sup> Liang Z. Tan,<sup>2</sup> Elio  
Champenois,<sup>3,4</sup> Said Bakhti,<sup>1</sup> Pavan Muddukrishna,<sup>1</sup> Thorsten Weber,<sup>1</sup>  
Ali Belkacem,<sup>1</sup> Daniel S. Slaughter,<sup>1,\*</sup> and Niranjana Shivaram<sup>1,†</sup>

<sup>1</sup>*Chemical Sciences Division, Lawrence Berkeley  
National Laboratory, Berkeley, CA 94720 USA*

<sup>2</sup>*Molecular Foundry, Lawrence Berkeley National Laboratory, Berkeley, CA 94720 USA*

<sup>3</sup>*Chemical Sciences Division, Lawrence Berkeley National Laboratory, Berkeley, CA 94720*

<sup>4</sup>*Graduate Group in Applied Science and Technology,  
University of California, Berkeley, CA 94720*

## Abstract

This supporting material provides details about Equation 1 in the main manuscript, the curve fitting of the UTPS data, evidence for two-photon absorption of the pump pulse by the nitrobenzene target, and the calculations of the ground and excited state third-order non-linear response.

## Measured UTPS signal:

The measured signal  $I_{raw}$  in our homodyne UTPS experiment, given by Equation 1, can be expanded as:

$$\begin{aligned}
I_{raw}(\tau, T) &= \int \left| E_{sig,A}(\omega, \tau, T) \right|^2 d\omega \\
&= \int \left[ |\chi_{eff,g}^{(3)}(\omega, \tau)|^2 |E_B(\omega)|^4 |E_A(\omega)|^2 + |\chi_{eff,g}^{(3)}(\omega, T)|^2 |E_{pump}(\omega)|^4 |E_A(\omega)|^2 \right. \\
&\quad + |\chi_{eff,ex}^{(3)}(\omega, \tau, T)|^2 |E_B(\omega)|^4 |E_A(\omega)|^2 + \chi_{eff,g}^{(3)}(\omega, \tau) \chi_{eff,g}^{(3)}(\omega, T)^* |E_B(\omega)|^2 |E_{pump}(\omega)|^2 |E_A(\omega)|^2 \\
&\quad + \chi_{eff,g}^{(3)}(\omega, \tau) \chi_{eff,ex}^{(3)}(\omega, \tau, T)^* |E_B(\omega)|^4 |E_A(\omega)|^2 \\
&\quad \left. + \chi_{eff,g}^{(3)}(\omega, T) \chi_{eff,ex}^{(3)}(\omega, \tau, T)^* |E_{pump}(\omega)|^2 |E_B(\omega)|^2 |E_A(\omega)|^2 + c.c \right] d\omega
\end{aligned} \tag{S1}$$

where  $c.c$  represents complex conjugate, and all constants have been absorbed into the susceptibilities. The time delay dependence of the spectral amplitudes appears as phase terms that disappear upon simplification and hence are not included here. Since we perform a lock-in measurement that measures signal only when the pump beam is present, the first term in equation S1 is not present. We also subtract signal measured when one of the probing pulses is blocked (probe B is blocked when measuring probe A signal). This removes the second term in equation S1. After these subtractions and further simplification, the processed signal  $I_{proc}$  can be written as,

$$\begin{aligned}
I_{proc}(\tau, T) &= a_1 |\chi_{eff,ex}^{(3)}(\tau, T)|^2 + a_2 \chi_{eff,g}^{(3)}(\tau) \chi_{eff,g}^{(3)}(T)^* + a_1 \chi_{eff,g}^{(3)}(\tau) \chi_{eff,ex}^{(3)}(\tau, T)^* \\
&\quad + a_2 \chi_{eff,g}^{(3)}(T) \chi_{eff,ex}^{(3)}(\tau, T)^* + c.c \tag{S2}
\end{aligned}$$

where we have assumed that the third-order susceptibilities are constant within the bandwidth of our laser pulses.  $a_1$  and  $a_2$  are constants obtained after integration of the spectral amplitudes over frequency. We note that  $|E_{pump}|^2$  is larger than  $|E_A|^2$ ,  $|E_B|^2$  by a factor of 3 in our experiment and the third-order susceptibilities  $\chi_{eff}^{(3)}$  are proportional to the number of molecules in the focal volume. From measurements of the pump absorption, we estimate that a few percent of the molecules are excited, therefore the number of excited molecules is approximately two orders of magnitude smaller than the number of molecules in the ground electronic state. This allows us to drop terms containing  $a_1$  and write equation S2 as

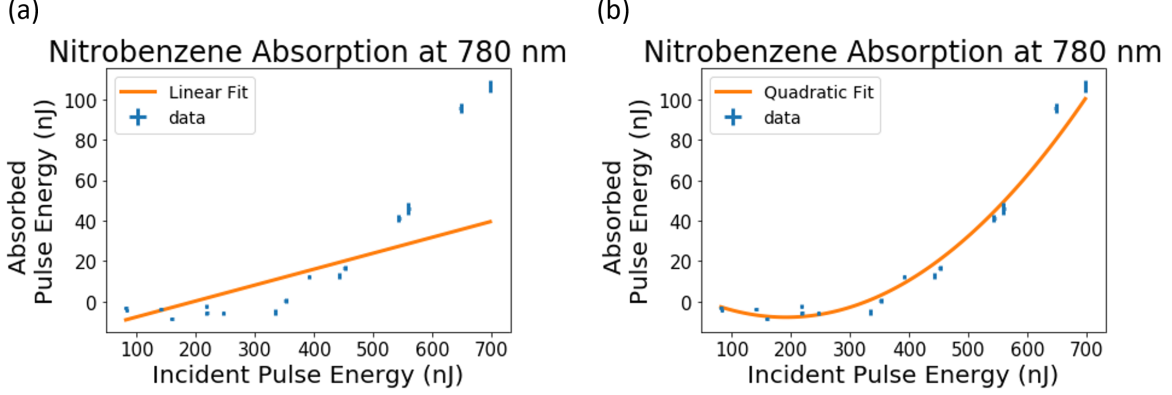

FIG. S1. (a) A plot of the absorbed pump pulse energy by the nitrobenzene target as a function of the incident pump pulse energy. A linear fit shown as orange solid line is not a good fit to the data. (b) Same data as in (a) but with a quadratic fit shown as the orange curve which fits the absorption data very well.

$$I_{proc}(\tau, T) \approx a_2 \chi_{eff,g}^{(3)}(\tau) \chi_{eff,g}^{(3)}(T)^* + a_2 \chi_{eff,g}^{(3)}(T) \chi_{eff,ex}^{(3)}(\tau, T)^* + c.c \quad (S3)$$

Here, we focus on the  $\tau$  and  $T$  dependent dephasing times which has contributions only from  $\chi_{eff,ex}^{(3)}(\tau, T)$ .

### Curve fitting:

The convolution shown in equation 2 in the manuscript can be written as

$$I_{sig}(\tau; T) = A_0 + A(T) \exp \left[ -\frac{(\tau - t_0(T))}{\gamma(T)} + \frac{1}{2} \left( \frac{\sigma}{\gamma(T)} \right)^2 \right] \text{erfc} \left[ \frac{1}{\sqrt{2}\sigma} \left( \frac{\sigma^2}{\gamma(T)} + t_0(T) - \tau \right) \right] \quad (S4)$$

where we have added an offset parameter  $A_0$  and  $\text{erfc}$  is the complementary error function. This equation is used in a curve-fitting procedure with  $\sigma = 30$  fs, which is obtained from the cross correlation measurement of the pulses using second harmonic generation.

## Two-photon absorption of the pump:

We have performed photo-absorption measurements of the pump beam, in order to verify that nitrobenzene is excited to the  $S_1$  state by two photon absorption of the pump pulse. Figure S1 shows the pump absorption data along with linear (Fig. S1 (a)) and quadratic (Fig. S1 (b)) fits. The good quadratic fit demonstrates that we are exciting nitrobenzene to the  $S_1$  state with a two-photon absorption. Our experimental pump pulse energy is around 430 nJ, well in the two-photon absorption regime.

## Target sample:

The target for our UTPS experiment is liquid nitrobenzene obtained from Sigma Aldrich (> 99% purity) and was used as received at room temperature.

## Calculation of $\chi_{eff}^{(3)}$ in the ground and excited states:

Calculations of  $\chi_{eff}^{(3)}$  of nitrobenzene were performed using the sum-over-states method [1, 2]. Molecular orbital energies and dipole matrix elements used in this sum were calculated within the density functional theory, with the B3LYP exchange correlation functional, norm-conserving pseudopotentials, and using the Quantum Espresso code [3]. Molecular geometries for these calculations were taken from Ref. [4]. The sum-over-states was performed as a sum over molecular orbitals, by assuming a single Slater determinant, and using a total of 82 molecular orbitals.  $\chi_{eff}^{(3)}$  calculations were performed for the electronic ground state and the excited  $S_1$  and  $T_2$  states. For the excited states, the Slater determinant with the highest weight was used, which was HOMO-3 $\rightarrow$ LUMO for  $S_1$  and HOMO-2 $\rightarrow$ LUMO for  $T_2$  [5]. To account for the random orientation of molecules in isotropic media, we take  $\chi_{eff}^{(3)} = \chi_{xyyx}^{(3)} + \chi_{xyxy}^{(3)}$  [6].

---

\* dsslaughter@lbl.gov

† niranjan@purdue.edu

[1] M. Nakano and K. Yamaguchi, Chemical Physics Letters **206**, 285 (1993).

- [2] B. M. Pierce, The Journal of Chemical Physics **91**, 791 (1989).
- [3] P. Giannozzi, S. Baroni, N. Bonini, M. Calandra, R. Car, C. Cavazzoni, D. Ceresoli, G. L. Chiarotti, M. Cococcioni, I. Dabo, A. D. Corso, S. d. Gironcoli, S. Fabris, G. Fratesi, R. Gebauer, U. Gerstmann, C. Gougoussis, A. Kokalj, M. Lazzeri, L. Martin-Samos, N. Marzari, F. Mauri, R. Mazzarello, S. Paolini, A. Pasquarello, L. Paulatto, C. Sbraccia, S. Scandolo, G. Sclauzero, A. P. Seitsonen, A. Smogunov, P. Umari, and R. M. Wentzcovitch, Journal of Physics: Condensed Matter **21**, 395502 (2009).
- [4] A. Giussani and G. A. Worth, J. Chem. Theory Comput. **13**, 2777 (2017).
- [5] J.-M. Mewes, V. Jovanović, C. M. Marian, and A. Dreuw, Phys Chem Chem Phys **16**, 12393 (2014).
- [6] T. R. Dickson, *Time-Resolved Optical Kerr Effect Spectroscopy by Four-Wave Mixing*, Ph.D. thesis, UNIVERSITY OF TORONTO (CANADA). (1991).
